# Supplementary material for: Best of Both Worlds Policy Optimization
Source: arXiv:2302.09408 source file (2023-02-18)
Supplement: Supplementary file 1 [file appendix-linear.tex]

\section{Analysis Linear MDP}
\textbf{Notation.}
Instead of considering states, I assume a state is defined by the action set $\calA$ that is currently available. So $\phi\in\calA$ can be seen as $\phi(a,s)$ in typical notation. W.l.o.g. I assume the actions are divided by stages, so $\calA\in\calS_h$ means that this is a action set we can encounter in stage $h$.
For a policy $\pi$, a state-action $\phi$ and an initial state-action $\phi_0$, I use $\mu_\pi(\phi;\phi')$ to denote the occupancy measure of $\phi$ after following a trajectory beginning by taking state-action $\phi'$. Without $\phi'$ this denotes the canonical starting state-action. By abuse of notation $\mu(\calA)$ denotes the measure of observing the ``state'' $\calA$. I use sums but can be thought of as integrals for non-countable sets.

For the information matrices, we use the following convention
\begin{align}
    &H_t(\calA) = \sum_{\phi\in\calA}\pi_t(\phi;\calA)\phi\phi^\top\\
    &\calH_{t,\pi,h} = \sum_{\calA\in\calS_h}\mu_\pi(\calA)H_t(\calA)\\
    &\calH_{t,h,\phi}=\sum_{\calA\in\calS_h}\mu_{\pi_t}(\calA;\phi)H_t(\calA)\label{eq: H from point}\\
    &\calH_{t,h} =\calH_{t,\pi_t,h} \label{eq: H policy}\,.
\end{align}
We denote the mixed policy
\begin{align*}
\pi^*_{t,h}(\cdot\,|\,\calA) := 
\begin{cases}
\pi^*(\cdot\,|\,\calA)&\text{ if }\calA\in\calS_{h'}\text{ for }h'<h\\
\pi_t(\cdot\,|\,\calA)&\text{ otherwise.}
\end{cases}
\end{align*}
\subsection{Preliminary logdet results}
For a trajectory of losses $\hatQ_t$ and a fixed action set $\calA\in\calS_h$, the regret of logdet barrier FTRL is bounded by
\begin{align*}
    &\E\left[\sum_{t=1}^T\inner{\bar\mu(\pi_t(\calA))-\phi^*,\hatQ_t}\right]\\
    &\leq \E\left[\sum_{t=1}^T\left(\eta\norm{\hat Q_t}^2_{H_t(\calA)} - B_t(\phi^*) + \E_{\phi\sim\pi_t(\calA)}[B_t(\phi)\right]\right)+\frac{d\log(T)}{\eta}+1\,.
\end{align*}
By using $\norm{\hat Q_t}^2_{H_t(\calA)}=\tr\left(\hat Q_t\hat Q_t^\top H_t(\calA)\right)$, $\hat Q_t = \calH_{t,h}^{-1}\phi_t L_{t,h}$, we have
\begin{align*}
    &\E_t[\norm{\hat Q_t}^2_{H_t(\calA)}]\\
    &\leq H^2\tr\left(\calH_{t,h}^{-1}\phi_t\phi_t^\top \calH_{t,h}^{-1} H_t(\calA)\right)]=H^2\tr(\calH_{t,h}^{-1}H_t(\calA))\,.
\end{align*}
With respect to the bias terms, note that
\begin{align*}
    &\sum_{\calA\in\calS_h}\mu_{\pi^*}(\calA)B_t(\phi^*) = \eta H^2\sum_{h'=h+1}^{H-1}\tr(\calH_{t,h}^{-1}\calH_{t,\pi^*_{t,h+1},h'})\\
    &\sum_{\calA\in\calS_h}\mu_{\pi^*}(\calA)\E_{\phi\sim \pi_t(\calA)}[B_t(\phi)]=\eta H^2\sum_{h'=h+1}^{H-1}\tr(\calH_{t,h}^{-1}\calH_{t,\pi^*_{t,h},h'})\,.
\end{align*}
\subsection{Main analysis}
It is easy to see that the Q-function estimates are unbiased, hence we have
\begin{align*}
    &\E\left[
    \sum_{t=1}^T\sum_{h=0}^{H-1}
    \sum_{\calA\in\calS_h}\mu_{\pi^*}(\calA)\sum_{\phi\in\calA}\left(\pi_t(\phi)-\pi^*(\phi)\right)\inner{\phi,Q^{\pi_t}_h}
    \right]\\
    &=\E\left[
    \sum_{t=1}^T\sum_{h=0}^{H-1}
    \sum_{\calA\in\calS_h}\mu_{\pi^*}(\calA)\sum_{\phi\in\calA}\left(\pi_t(\phi)-\pi^*(\phi)\right)\inner{\phi,\hatQ_t}
    \right]\\
    &\leq \E\left[\sum_{t=1}^T\sum_{h=0}^{H-1}
    \sum_{\calA\in\calS_h}\mu_{\pi^*}(\calA)\eta\left(\norm{\hatQ_t}_{H_{t}(\calA)}^2-B_t(\phi^*)+E_{\pi_t}[B_t(\phi)]\right)
    \right]+\frac{dH\log(T)}{\eta}\\
    &= \E\left[\sum_{t=1}^T\sum_{h=0}^{H-1}\eta H^2\left(
    \tr(\calH^{-1}_{t,h}\calH_{t,\pi^*_{t,h},h})-\sum_{h'=h+1}^{H-1}\left(\tr(\calH^{-1}_{t,h'}\calH_{t,\pi^*_{t,h+1},h'})-\tr(H^{-1}_{t,h'}H_{t,\pi^*_{t,h},h'})\right)\right)
    \right]+\frac{dH\log(T)}{\eta}\\
    &= \E\left[\sum_{t=1}^T\sum_{h=0}^{H-1}\eta H^2
    \tr(\calH^{-1}_{t,h}\calH_{t,h})
    \right]+\frac{dH\log(T)}{\eta}\\
    &= \eta d T H^3 +\frac{dH\log(T)}{\eta}
\end{align*}
